# Supplementary material for: Live Long and Prosper:Analyzing Long-Lived MOAS Prefixes in BGP
Source: arXiv:2307.08490 source file (2023-07-17)
Supplement: Supplementary file 1 [file appendix.tex]

%! TEX root = ../paper.tex

\clearpage

\section{appendix}
\label{appendix:definition}

\subsection{}
From 2017 to 27 September 2022
We observe a total of 169311 and 13691 IPv4 and IPv6 MOAS prefixes on the Internet, respectively. Only 70418 IPv4 and 5225 IPv6 MOAS live minimum 30 days.
The knee value for IPv4 is 30 days, for IPv6, it is 26 days and together 38 days is the knee value of the data. We use the “S” sensitivity value of “1” day for our analysis.
We extract all MOAS prefixes that lived a minimum of 30 days (i.e., knee value of maximum MOAS prefix life) and apply further analysis
